# Supplementary material for: Unsupervised Opinion Summarization as Copycat-Review Generation
Source: arXiv:1911.02247 source file (2020-04-19)
Supplement: Supplementary file 1 [file ablation_summs.tex]

% B003YJ5LLM

\begin{table*}
 	\footnotesize 
 	\centering
    \begin{tabular}{ | c | p{12cm} |}
    \hline
     & \multicolumn{1}{>{\centering}m{110mm}|}{Summary} \\ \hline
    Full & This is a great case for the Acer Aspire 14' laptop. It is a little snug for my laptop, but it's a nice case. I would recommend it to anyone who wants to protect their laptop.\\ \hline
    w/o $r_{\_i}$ & This is the best case for the money. The sleeve is a little too bulky but it 's nice to be able to carry it on my laptop. I recommend it to my friends.\\ \hline
    w/o $c$ &  I love this case. It is perfect for my Acer Aspire one. It is a little snug but that's why I bought it for my laptop. I love it and recommend it.\\ \hline
    w/o $z$ & This is a great case, but I had to return it. I returned it for a refund because it was damaged when I received it. The case is the only reason I gave it 4 stars instead of 5 stars because of the price.\\ \hline 
    & \multicolumn{1}{>{\centering}m{110mm}|}{Input}\\ \hline
    Review 1 & Love the design of this sleeve. When I don't have a table I use the sleeve as a mat to protect my thighs from the heat of my laptop. Wish it had a bit more padding and cushion but other than that it's a pretty carrying sleeve.\\ \hline
    Review 2 & This was bought for our teen daughter for Christmas, the only negative things about it are 1.no strap 2.no pockets, other than that it is great, but in all fairness i knew both things about it when ordered, it came in very fast, was just as described, great item for the price.\\ \hline
    Review 3 & This case fits perfectly on my 14inch hp. I disagree with the comments that talk about the smell being terrible. The smell really wasn't that strong and went away after a couple of weeks. I love the design and it was a fair price. Shipping was a little expensive though. It arrived quickly and I would buy from this seller again.\\ \hline
    Review 4 & I really enjoy the design of this case but I thought it would be lighter. When it came, it was a very dark grey which was a bummer. But the quality is good and it has a nice thick padding to protect my laptop.\\ \hline
    Review 5 & I like this case very much! It fits my Acer Aspire 14 'as a glove!!! Yes, it smells a little bit but I wouldn't say that it's so bad as mentioned in some reviews. And it's very cute too. I recommend this product to anyone.\\ \hline
    Review 6 & I BOUGHT IT FOR MY ACER 14 ', IT IS A LITTLE BIT TIGHT, BUT THE WORST WAS IT HAS HEAVY RUBBER SMELL, WHEN I LEAVE THE CASE IN MY ROOM, THE RUBBER SMELL WAS FILLED WITH THE AIR EVERYWHERE OF MY ROOM, MADE ME SICK. DON'T BUY IT.\\ \hline
    Review 7 & I have a dell inspiron 14, and the cover is a little snug. It's working well though and now I can carry my laptop in my school backpack rather than carry a separate laptop bag. I'd recommend this product, just do a bunch of research to make sure it will fit.\\ \hline
    Review 8 & I really love it! It doesn't smell a lot as some reviews say and the draw is well defined.I bought this size for a 13.3 'because my laptop will have a cover on it so I don't know how it fits for a traditional 14 inch,\\ \hline
    \end{tabular}
    \caption{Amazon summaries of the ablated model.}
    \label{table:ama_ablation_summs1}
\end{table*}
