# Supplementary material for: Unsupervised Opinion Summarization as Copycat-Review Generation
Source: arXiv:1911.02247 source file (2020-04-19)
Supplement: Supplementary file 2 [file latent_vars_penalty.tex]

\subsection{Latent Variables Penalty}
To investigate the effect that the latent codes penalty has on the model, we experimented with different annealing maximum penalties for the latent codes $c$. Specifically, we fixed the maximum penalty scalar for the $z$ associated KLD to 1., and varied the maximum penalty scalar for the $c$ associated KLD term $\alpha$. The variable $c$ models the group representations, which are used to condition the prior $p_{\theta}(z|c)$. Consequently, it directly affects the flexibility of the latent space of $z$. The results in terms of the averaged lower bound components on the unlabelled validation set are shown in Table \ref{table:c_max}.

\begin{table*}[h!]
\centering
    \begin{tabular}{ | c | c | c | c | N |}
    \hline
     max $\alpha$ & $\log p_{\theta}(r_i | z, r_{\_i})$ & $\KL{q_{\phi}(c| \cdot)}{p_{\theta}(c)}$  & $\KL{q_{\phi}(z | \cdot)}{p_{\theta}(z| \cdot)}$ & \\[10pt] \hline
     0.1 & -96.63 & 1575.66 & 14.44 & \\ \hline
     0.3 & -149.09 & 209.77 & 17.83 & \\ \hline
     0.5 & -157.83 & 59.36 & 19.24 & \\ \hline
     0.7 & -159.39 & 30.33 & 19.05 & \\ \hline
    \end{tabular}
    \caption{The effect of the maximum annealing penalty for the group latent code $c$ on the lower bound.}
    \label{table:c_max}
\end{table*}

We observed that the lower penalty of the $c$'s KLD results in better reconstruction of reviews and more diverse summaries, the former observation is consistent with \citep{shen2019latent}. Intuitively, the model is able to store more information about the group into the variable, and produce a less restricted prior over $z$. However, we noticed that $\alpha=0.1$ sometimes leads to generation of less fluent and incomplete sentences. It can be explained by the fact that the latent space of $z$ gets less restricted, and receives a sparser coverage during training. Also, the maximum penalty does not affect the divergence of the posterior $q_{\phi}(z| r_i, c)$, which indicates that

Finally, we observed an increase of the amount of generated repetitions both in the reconstructed reviews and summaries in the end of annealing cycles for higher values of $\alpha$. It can be explained by the fact that at the end of cycles, the model receives a higher penalty for storing information into the latent codes. Consequently, the initial hidden state of the decoder becomes less informative, and it starts relying on local statistics of the language model to perform reconstruction. Our observations are somewhat aligned to the language models associated repetitions discussed in \citep{holtzman2019curious}.
